# Supplementary material for: The eMERGE Survey I: Very Large Array 5.5 GHz observations of the GOODS-North Field
Source: arXiv:1705.03766 source file (2017-05-10)
Supplement: Supplementary file 1 [file appendix.pdf]

## APPENDIX A: RADIO CONTOUR PLOTS OF THE SOURCES DETECTED AT 5.5 GHZ

This appendix contains the postage-stamp images of the 94 radio sources detected at 5.5 GHz.

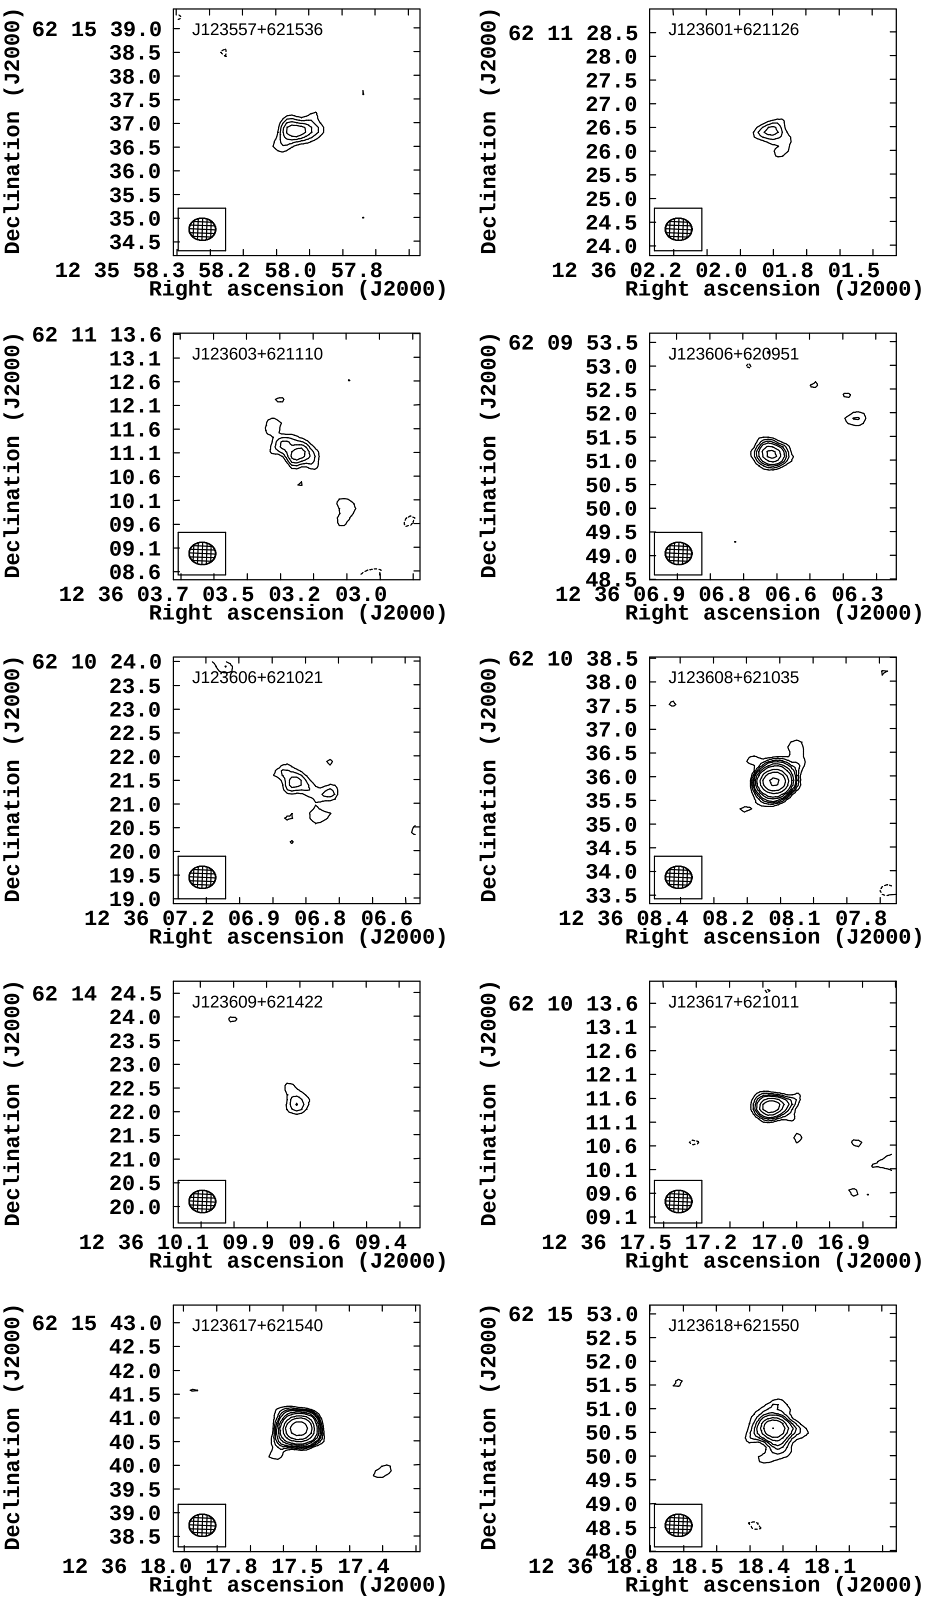


**Figure A1.** Online version only: contour plots at 5.5 GHz. Levels are $-3, 3, 4, 5, 6, 8, 10, 15, 25, 50, 100, 250, 500 \times \sigma$, where $\sigma$ is the local r.m.s. noise. The FWHM beam size is plotted in the bottom-left corner. Each postage-stamp is 5 arcsec on-the-side, with the exception of J123644+621133 (15 arcsec) and J123726+621128 (10 arcsec).

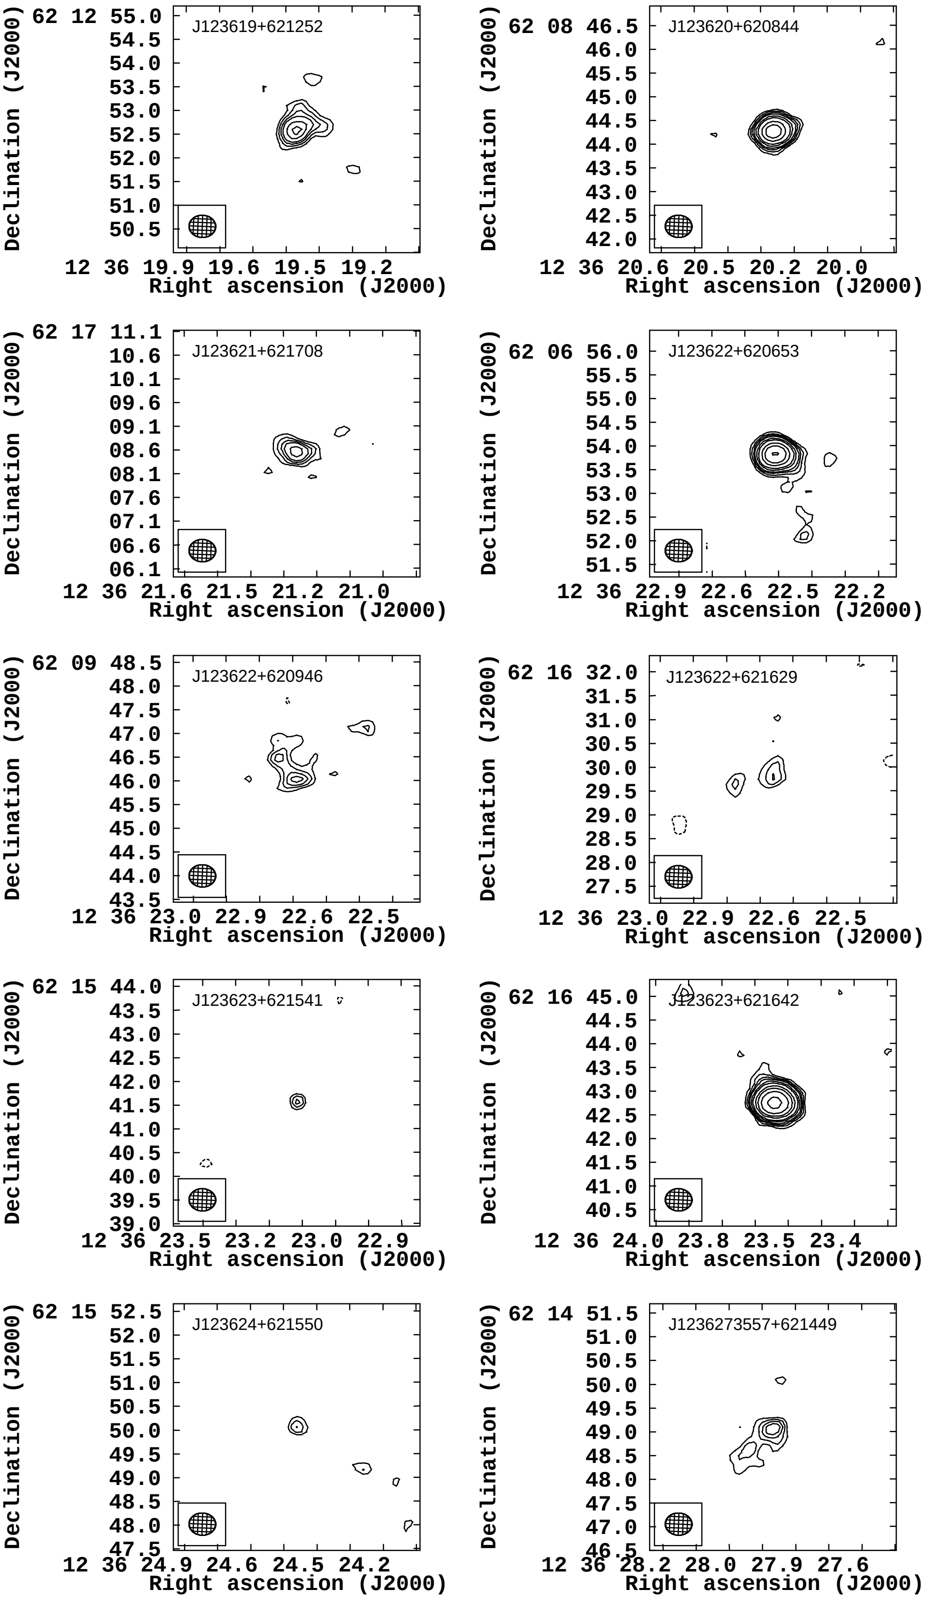


**Figure A1** – *continued* Contour plots at 5.5 GHz

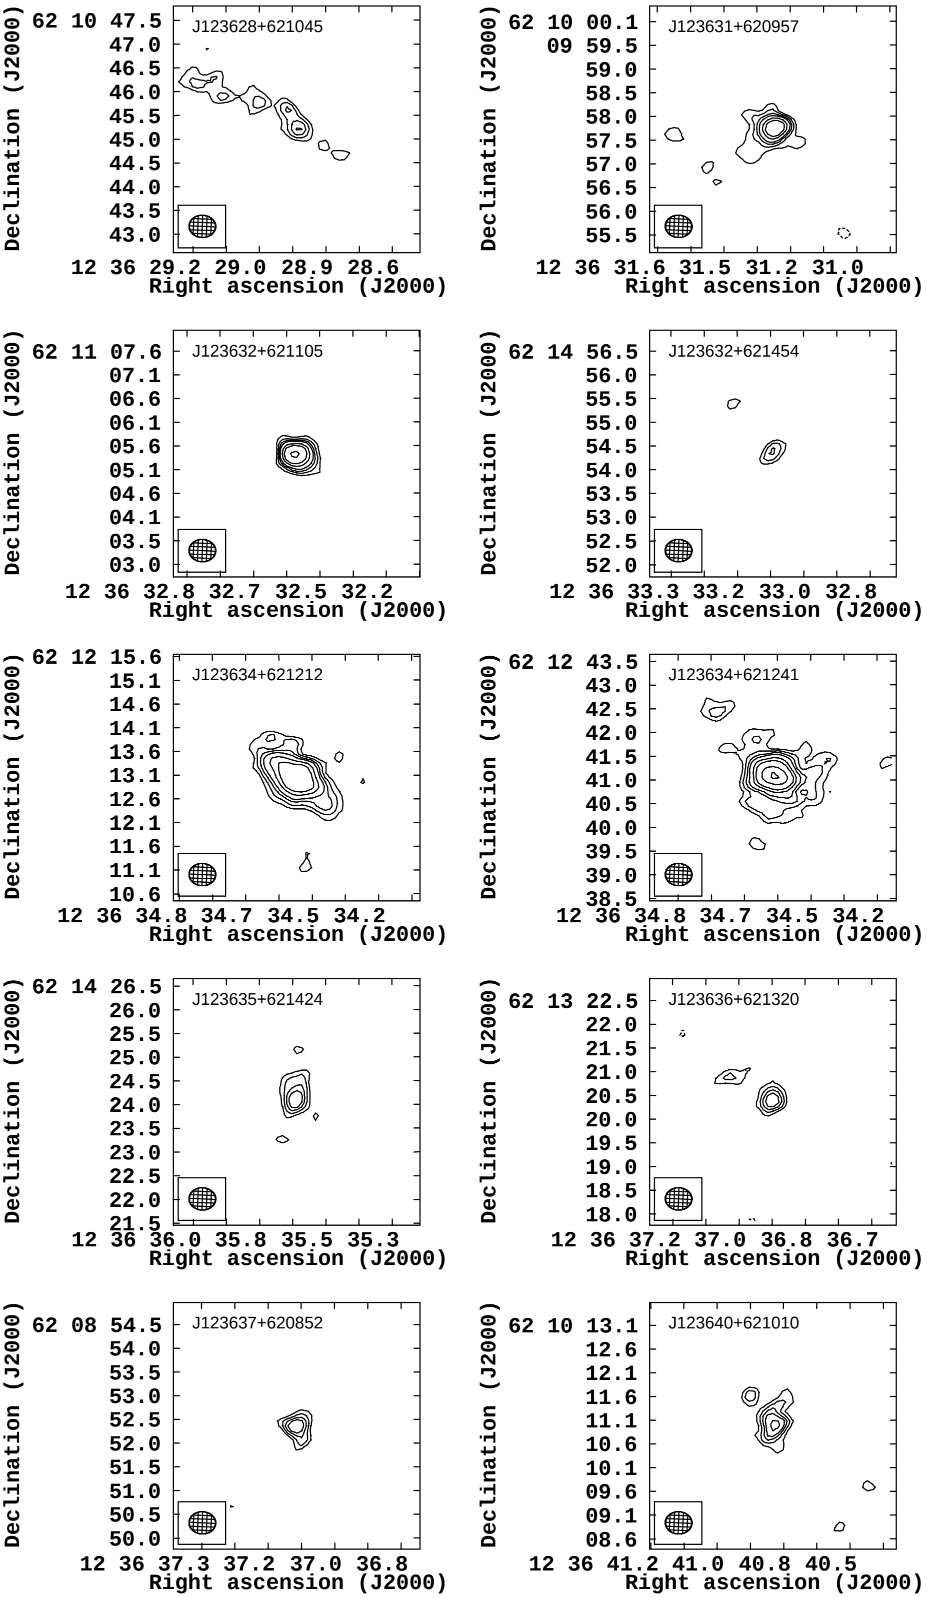


**Figure A1** – *continued* Contour plots at 5.5 GHz

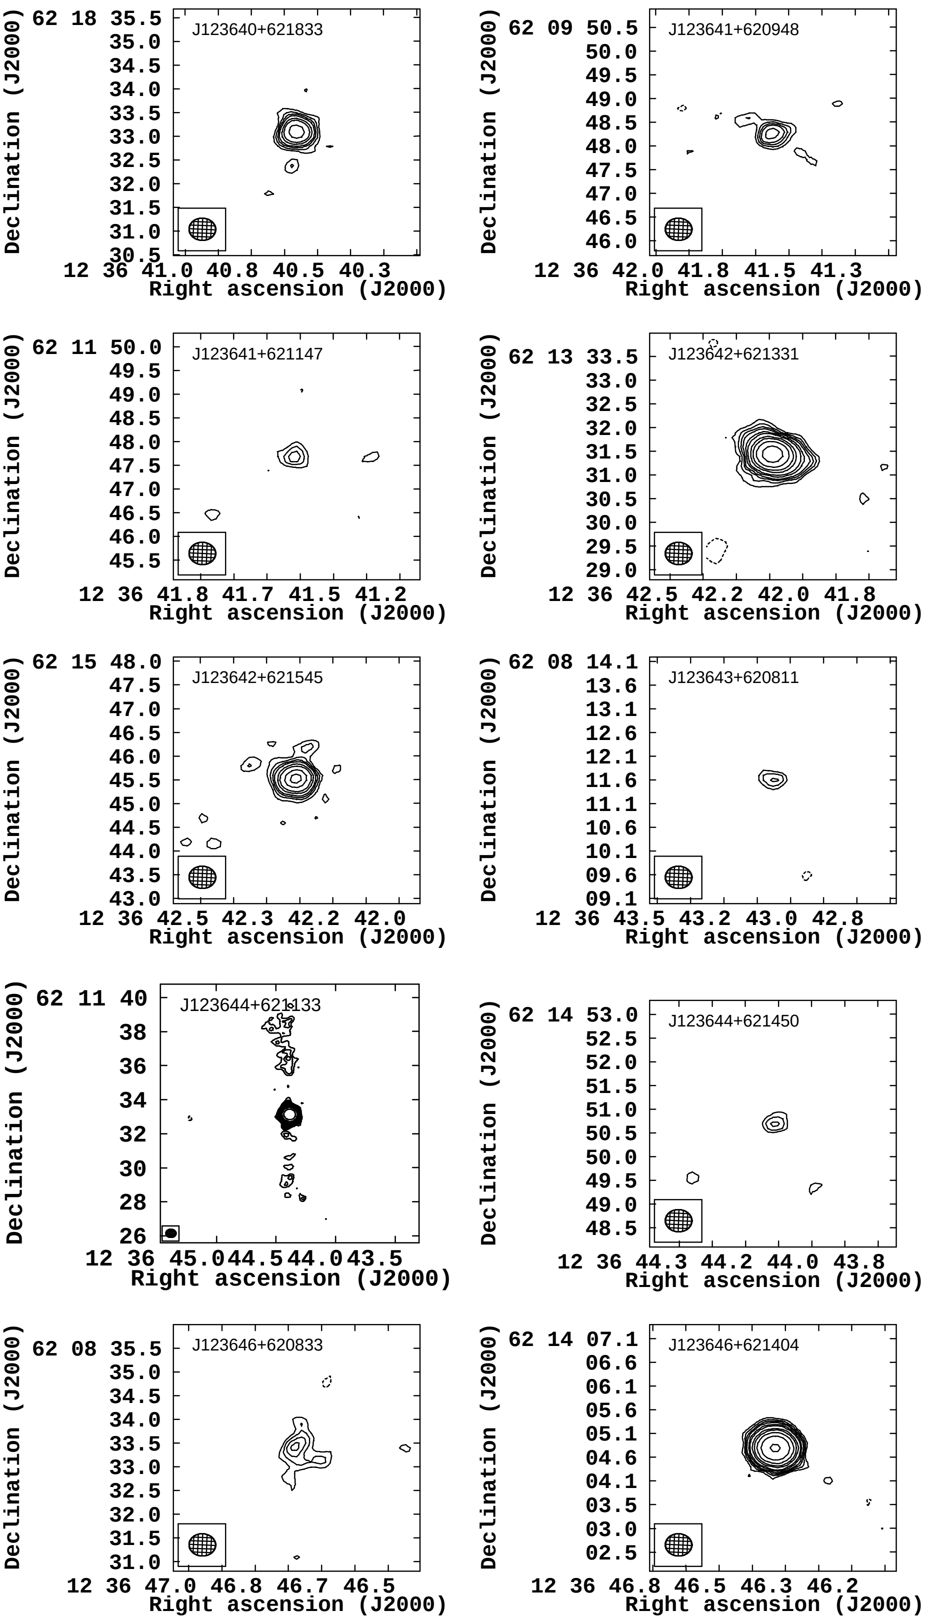


**Figure A1** – *continued* Contour plots at 5.5 GHz

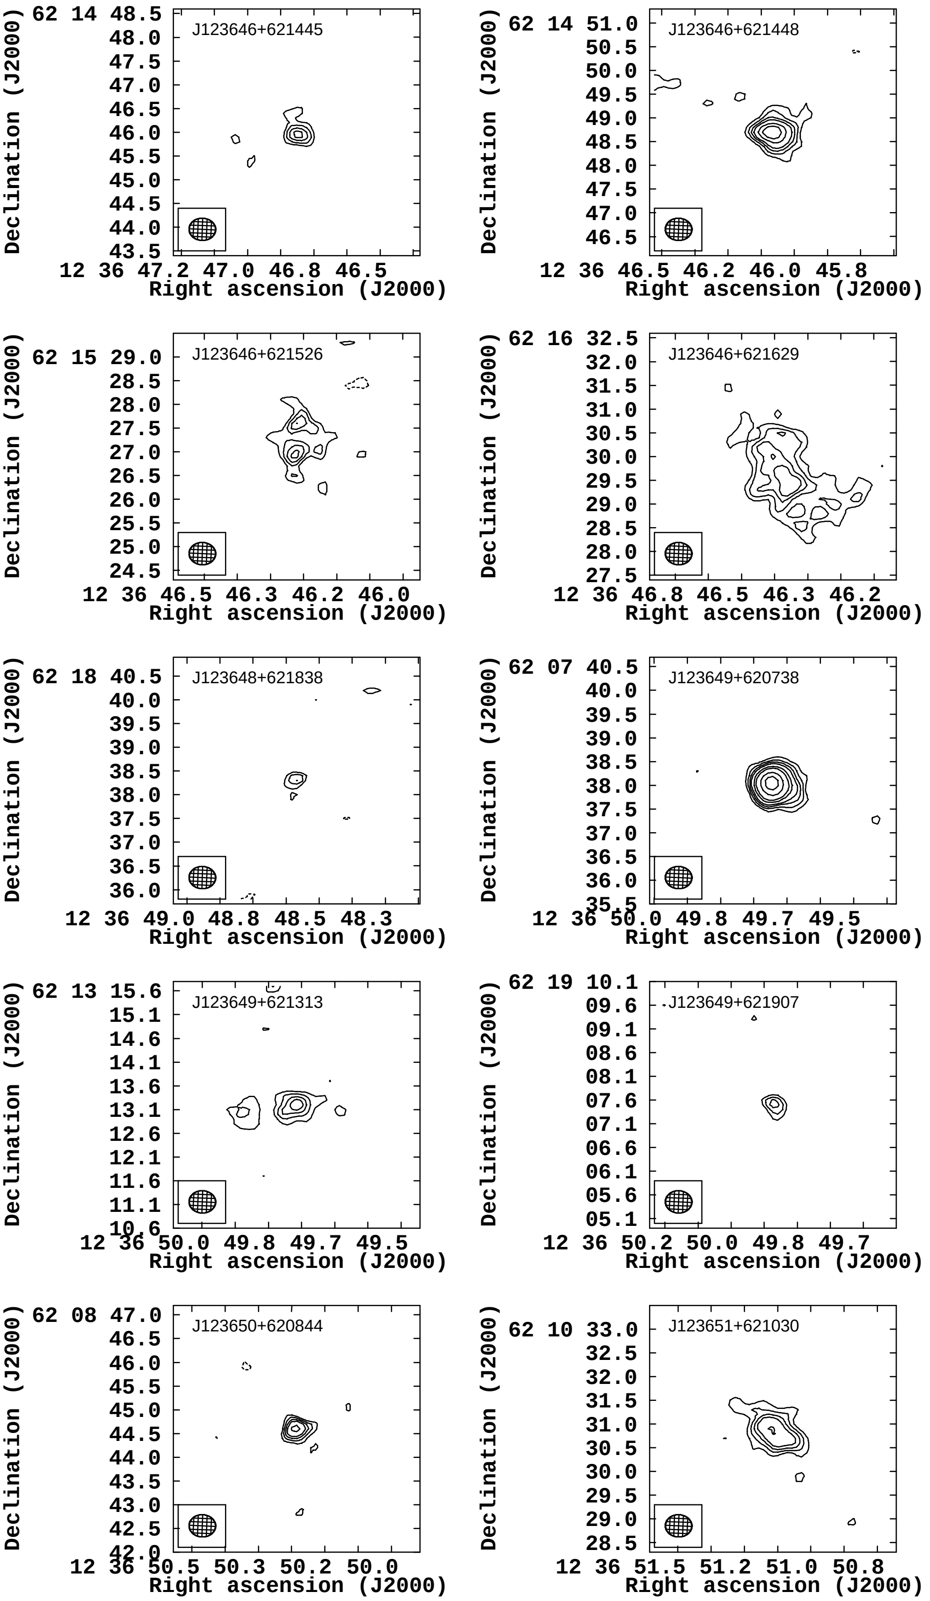


**Figure A1** – *continued* Contour plots at 5.5 GHz

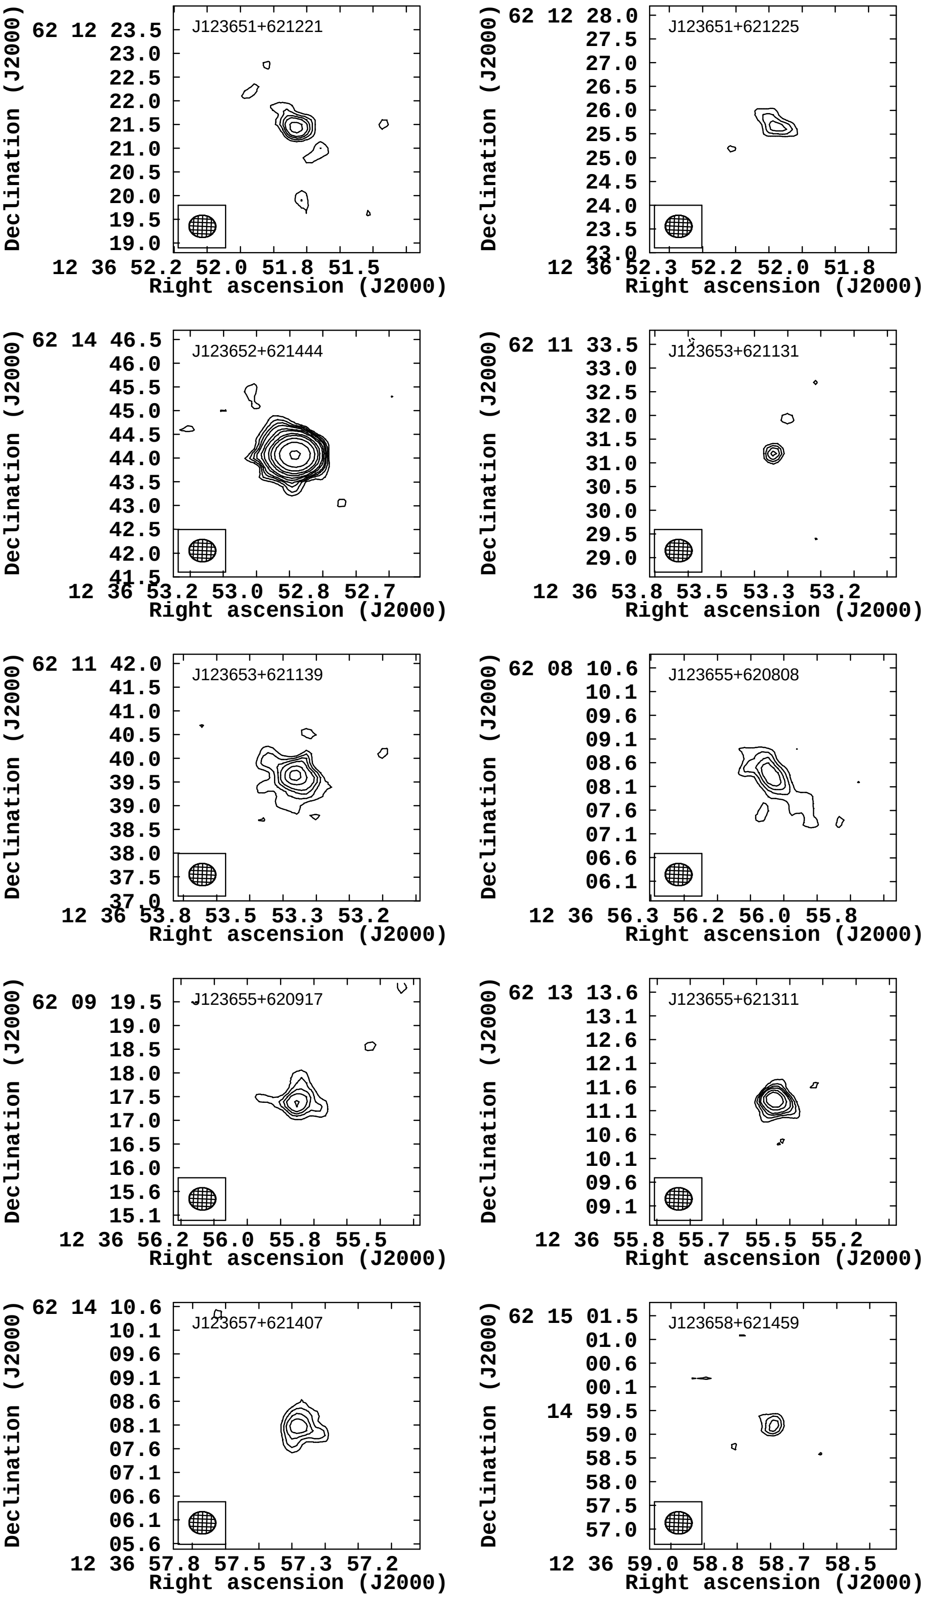


**Figure A1** – *continued* Contour plots at 5.5 GHz

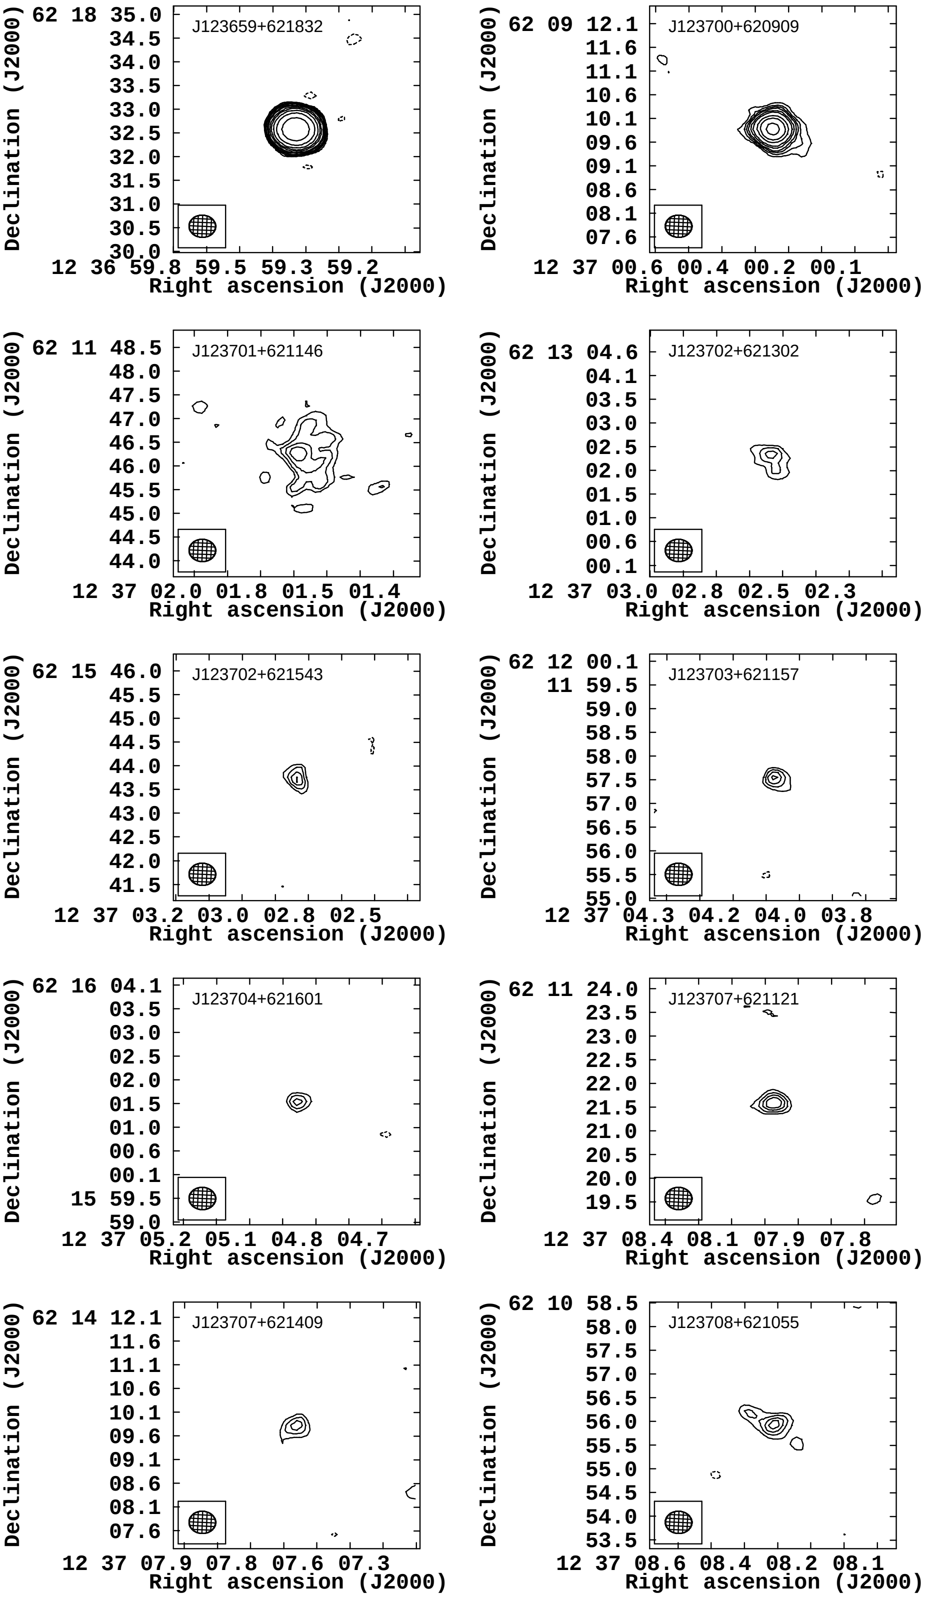


**Figure A1** – *continued* Contour plots at 5.5 GHz

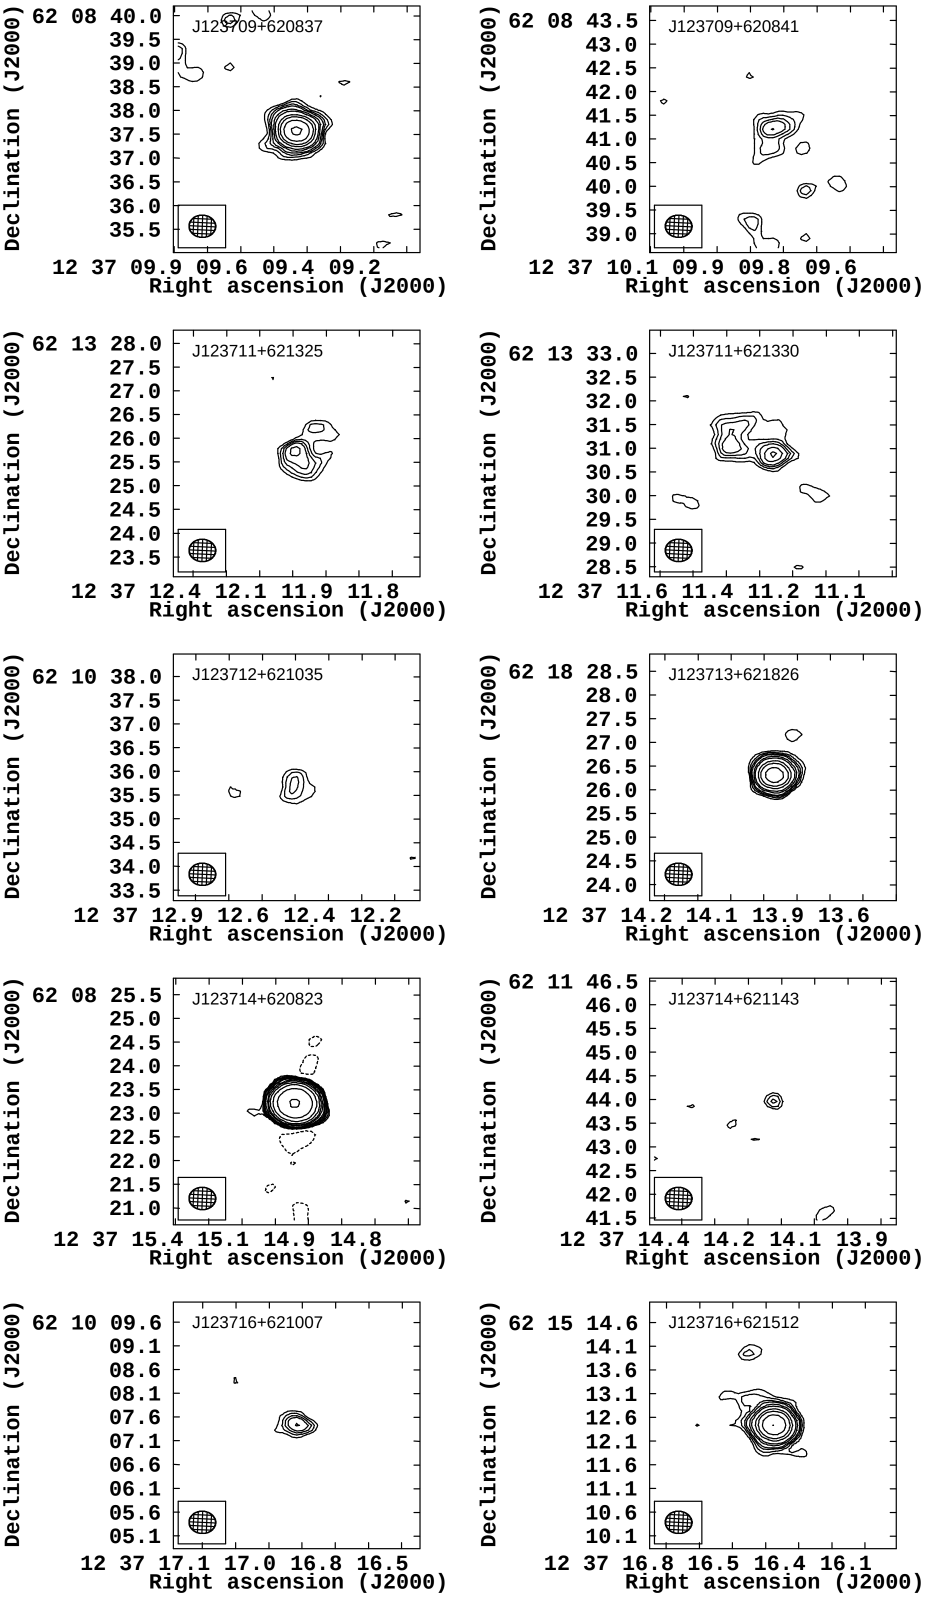


**Figure A1** – *continued* Contour plots at 5.5 GHz

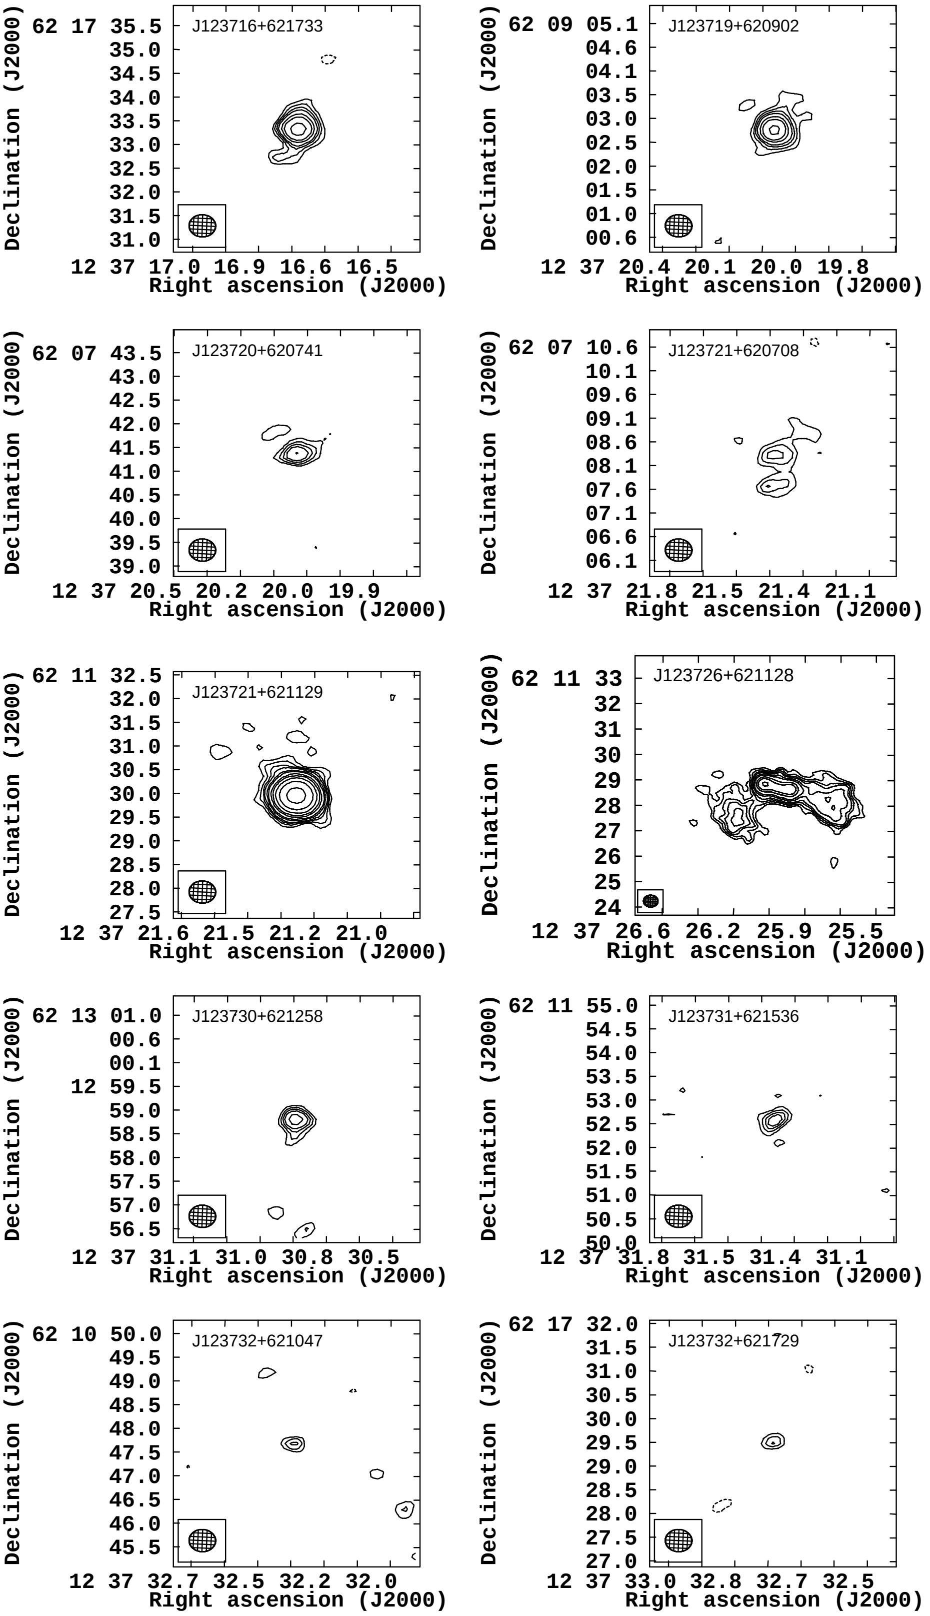


**Figure A1** – *continued* Contour plots at 5.5 GHz

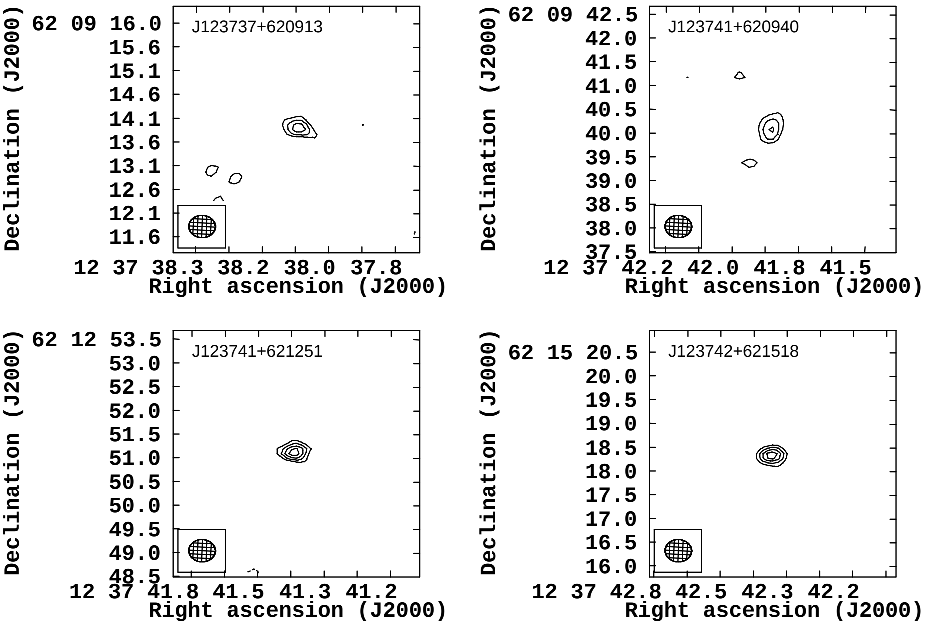


**Figure A1** – *continued* Contour plots at 5.5 GHz
